# Supplementary material for: OmniSeg3D: Omniversal 3D Segmentation via Hierarchical Contrastive Learning
Source: arXiv:2311.11666 source file (2023-11-20)
Supplement: Supplementary file 1 [file X_suppl.tex]

\clearpage
\setcounter{page}{1}
\maketitlesupplementary

\section{Rationale}
\label{sec:rationale}
Having the supplementary compiled together with the main paper means that:
\begin{itemize}
\item The supplementary can back-reference sections of the main paper, for example, we can refer to \cref{tab:hierarchy};
\item The main paper can forward reference sub-sections within the supplementary explicitly (e.g. referring to a particular experiment); 
\item When submitted to arXiv, the supplementary will already included at the end of the paper.
\end{itemize}
To split the supplementary pages from the main paper, you can use \href{https://support.apple.com/en-ca/guide/preview/prvw11793/mac#:~:text=Delete%20a%20page%20from%20a,or%20choose%20Edit%20%3E%20Delete).}{Preview (on macOS)}, \href{https://www.adobe.com/acrobat/how-to/delete-pages-from-pdf.html#:~:text=Choose%20%E2%80%9CTools%E2%80%9D%20%3E%20%E2%80%9COrganize,or%20pages%20from%20the%20file.}{Adobe Acrobat} (on all OSs), as well as \href{https://superuser.com/questions/517986/is-it-possible-to-delete-some-pages-of-a-pdf-document}{command line tools}.

\section{Details on Quantitative Results}

\haiyang{When illustrating the formulation, remember to explain why we use \textbf{xyz} and why using it is an appropriate option since SA3D~\cite{cen2023samin3d} didn't use this. 
An intuition explanation may be:
We optimize segmentation information for everything simultaneously in the 3D space instead of single object.
}

We retrieve the volume rendered feature maps $\V{f}$ (with unit norm) from the reference and target views, and compute the spatial coordinate $\V{x}$ corresponding to each pixel $\V{p}$ from the rendered depth. The similarity  between pixels $\V{p}_1$ and $\V{p}_2$ is defined as a distance-weighted feature similarity:
\begin{equation}
    \mathrm{sim}\,(\V{p}_1,\V{p}_2)=\exp{(-\alpha\norm{\V{x}_1-\V{x}_2})}\cdot(1+\V{f}_1\cdot\V{f}_2)
\end{equation}
where $\alpha$ is a positive constant depending on the spatial scale of the dataset. We sample positive pixels $\{\V{p}_i\,|\,i\in S_{pos}\}$ from the foreground scribble and negative pixels $\{\V{p}_j\,|\,j\in S_{neg}\}$ from the background scribble in the reference view. The score for each pixel $\V{p}_t$ in the target view is defined through the difference of maximal similarities with positive and negative samples:
\begin{equation}
    \mathrm{score}\,(\V{p}_t)=\max_{i\in S_{pos}}{\mathrm{sim}\,(\V{p}_t,\V{p}_i)}-\beta\max_{j\in S_{neg}}{\mathrm{sim}\,(\V{p}_t,\V{p}_j)}
    \label{eq:score}
\end{equation}
where $\beta=0.15$. In practice, the maximal similarity with positive samples is replaced by the 95th percentile to suppress noise. The predicted mask in the target view $\V{I}_{tgt}$ is then:
\begin{equation}
    M_{tgt}=\{\V{p}_t\in \V{I}_{tgt}\,|\,\mathrm{score}\,(\V{p}_t)>thresh\}
    \label{eq:thresh}
\end{equation}
where the threshold is automatically chosen from the reference view and kept constant for any target view.

Similar to the previous section, the score map for each view (including the reference view) is computed with Equation \ref{eq:score}, where positive and negative samples ($S_{pos}$ and $S_{neg}$) are drawn uniformly from the reference view according to the input mask $M_{GT}$. The binarization threshold in Equation \ref{eq:thresh} is determined by maximizing the IoU between the predicted and ground truth masks in the reference view $\V{I}_{ref}$:
$\max_{thresh}\mathrm{IoU}\,(\{\V{p}_t\in \V{I}_{ref}\,|\,\mathrm{score}\,(\V{p}_t)>thresh\},M_{GT})$,
then the same threshold is applied to all other views for evaluation.

\section{Typo Correction}
Some typos should be corrected as follows:

\vspace{6pt}
\noindent{\textbf{1. line 323 - 327, line 330}}. All the $l$ should be replaced with $d$ (means the depth of one patch in the hierarchy tree) for clearer explanation of the data structure. The \textit{patch index map} should be replaced with \textit{patch index set}. A patch index set $S_d^i$ stands for the index set of patches that at the depth $d$ of the hierarchy tree of patch $i$. For example, $S_{d=3}^{i=4}=\{2, 3\}$ in Fig.~2 of the main paper.

\begin{equation} \mathcal{L}_{H}=\sum_{i=1}^{N_p}\sum_{d=1}^{d^i_{max}} \frac{\lambda^{d-1}}{NL}\sum_{j=1}^{|\{\mathbf{f}^i\}|} \sum_{s\in S_d^i}  \max(\mathcal{L}^{i,j}(s),\mathcal{L}_{max}^{i,j}(d-1)) ,
% \label{eq:reg}
\end{equation}
where 
$S^i_d$ is the patch index set at level $d$ of anchor patch $i$, $ s\in S^i_d$ is a patch at depth $d$, 
$\mathcal{L}^{i,j}(s)$ is the contrastive loss between point $j$ (in point set of patch $i$) and the average feature $\bar{\mathbf{f}}^s$ of patch $s$:

\vspace{6pt}
\noindent{\textbf{2. line 330}}: The $l$ should be replaced with $d$:

\begin{equation}
    \mathcal{L}_{max}^{i,j}(d)=\max_{s\in S^i_d}\mathcal{L}^{i,j}(s).
\end{equation}

\section{Mesh-based Implementation}
As shown in the main paper, our method is also not restricted by the underlying 3D representations and can be easily extended to mesh based rendering pipeline. 
% Mesh segmentation is also a vital application scenario, especially compared to NeRF-based representation.
For mesh-based representation, we implement a rasterization-based rendering pipeline, in which only the points located on the mesh will be sampled for rendering optimization while the network architecture remains the same as the volume rendering pipeline in the main paper. 
Besides, we believe our OmniSeg3D will be a simple plug-in for point-based (like point-NeRF~\cite{} and Gaussian Spatting~\cite{})and SDF-based (like Neus~\cite{} and Neuralangelo~\cite{}) rendering pipelines.

\section{Alternative 2D segmentation methods}
We demonstrate the proposed methodology of OmniSeg3D is \textbf{a general paradigm} for lifting 2D inconsistent segmentation into 3D, instead of a method limited by any specific 2D segmentation methods.
Though we use SAM~\cite{kirillov2023sam} as 2D backbone in our implementation, any interactive or click-based segmentation methods like ~\cite{sofiiuk2022ritm, liu2023simpleclick, chen2022focalclick} can be used as our 2D backbone. 
Meanwhile, due the high dependence on multi-view consistent 2D segmentations, SA3D~\cite{cen2023samin3d} may be more strongly bound to SAM~\cite{kirillov2023sam}.

TODO: experiments.

\section{Automatic Discretization}
As a further explanation and discussion about Fig.~6 in the main paper.
